# Supplementary material for: Basis-set correction for coupled-cluster estimation of dipole moments
Source: arXiv:2202.12556 source file (2022-02-25)
Supplement: Supplementary file 1 [file supp_info.pdf]

# **Basis-set correction for coupled-cluster estimation of dipole moments**

## **Supplementary information**

Diata Traore\*

*Laboratoire de Chimie Thorique, Sorbonne Universit and CNRS, F-75005 Paris, France*

Julien Toulouse†

*Laboratoire de Chimie Thorique, Sorbonne Universit and CNRS, F-75005 Paris, France and  
Institut Universitaire de France, F-75005 Paris, France*

Emmanuel Giner‡

*Laboratoire de Chimie Thorique, Sorbonne Universit and CNRS, F-75005 Paris, France and*

(Dated: February 9, 2022)

---

\* diata.traore@upmc.fr

† toulouse@lct.jussieu.fr

‡ emmanuel.giner@lct.jussieu.fr

**CONTENTS**

|                                        |    |
|----------------------------------------|----|
| I. Geometries                          | 3  |
| II. Detailed results for the molecules | 4  |
| III. Table of errors                   | 18 |
| References                             | 18 |

## I. GEOMETRIES

TABLE I. Input xyz geometries (in angstrm) and their references.

| Molecules                     |         |         |         |
|-------------------------------|---------|---------|---------|
| CO [1]                        |         |         |         |
| C                             | 0.0000  | 0.0000  | 0.0000  |
| O                             | 0.0000  | 0.0000  | 1.1282  |
| BeH [1]                       |         |         |         |
| Be                            | 0.0000  | 0.0000  | 0.0000  |
| H                             | 0.0000  | 0.0000  | 1.3426  |
| BF [1]                        |         |         |         |
| B                             | 0.0000  | 0.0000  | 0.0000  |
| F                             | 0.00000 | 0.0000  | 1.2669  |
| BH [2]                        |         |         |         |
| B                             | 0.0000  | 0.0000  | 0.0000  |
| H                             | 0.0000  | 0.0000  | 1.2324  |
| CH [1]                        |         |         |         |
| C                             | 0.0000  | 0.0000  | 0.0000  |
| H                             | 0.0000  | 0.0000  | 1.1199  |
| NH [1]                        |         |         |         |
| N                             | 0.0000  | 0.0000  | 0.0000  |
| H                             | 0.0000  | 0.0000  | 1.0362  |
| CH <sub>2</sub> (singlet) [1] |         |         |         |
| C                             | 0.0000  | -0.0000 | 0.1734  |
| H                             | 0.0000  | -0.8623 | -0.5202 |
| H                             | 0.0000  | -0.8623 | -0.5202 |
| FH [2]                        |         |         |         |
| F                             | 0.0000  | 0.0000  | 0.0000  |
| H                             | 0.0000  | 0.0000  | 0.9170  |
| H <sub>2</sub> O [1]          |         |         |         |
| O                             | 0.0000  | 0.0000  | 0.1173  |
| H                             | 0.0000  | 0.7572  | -0.4692 |
| H                             | 0.0000  | -0.7572 | -0.4692 |
| BN [1]                        |         |         |         |
| B                             | 0.0000  | 0.0000  | 0.0000  |
| N                             | 0.0000  | 0.0000  | 1.3250  |
| BO [1]                        |         |         |         |
| B                             | 0.0000  | 0.0000  | 0.0000  |
| O                             | 0.0000  | 0.0000  | 1.2045  |
| LiH [1]                       |         |         |         |
| Li                            | 0.0000  | 0.0000  | 0.0000  |
| H                             | 0.0000  | 0.0000  | 1.5949  |
| LiF [1]                       |         |         |         |
| Li                            | 0.0000  | 0.0000  | 0.0000  |
| F                             | 0.0000  | 0.0000  | 1.5639  |
| LiN [1]                       |         |         |         |
| Li                            | 0.0000  | 0.0000  | 0.0000  |
| N                             | 0.0000  | 0.0000  | 1.8690  |

## II. DETAILED RESULTS FOR THE MOLECULES

TABLE II. CO

| Basis/Method | HF       | CCSD(T) | CCSD(T)+PBEUEG |
|--------------|----------|---------|----------------|
| aug-cc-pVDZ  | -0.10199 | 0.05550 | 0.04398        |
| aug-cc-pVTZ  | -0.10499 | 0.05000 | 0.04414        |
| aug-cc-pVQZ  | -0.10433 | 0.04600 | 0.04273        |
| aug-cc-pV5Z  | -0.10421 | 0.04500 | 0.04360        |
| CBS          |          | 0.04485 |                |

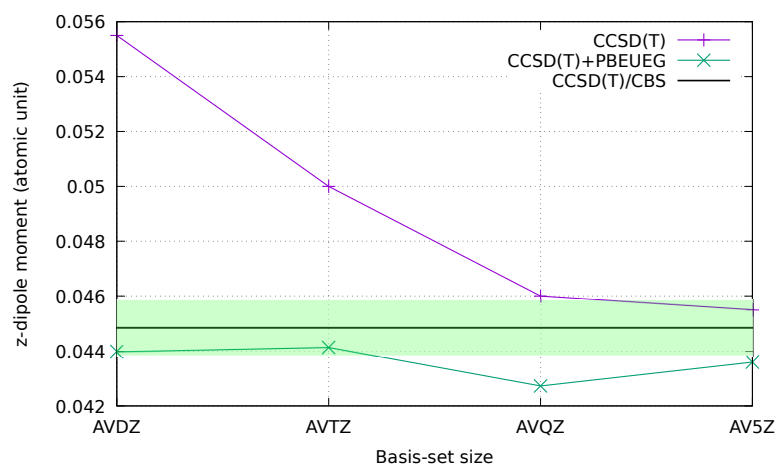

FIG. 1. CO

TABLE III. BeH

| Basis/Method | ROHF    | ROCCSD(T) | ROCCSD(T)+PBEUEG |
|--------------|---------|-----------|------------------|
| aug-cc-pVDZ  | 0.11017 | 0.09550   | 0.08416          |
| aug-cc-pVTZ  | 0.11076 | 0.09100   | 0.08746          |
| aug-cc-pVQZ  | 0.11199 | 0.09050   | 0.08941          |
| aug-cc-pV5Z  | 0.11218 | 0.09050   | 0.08980          |
| CBS          |         | 0.09030   |                  |

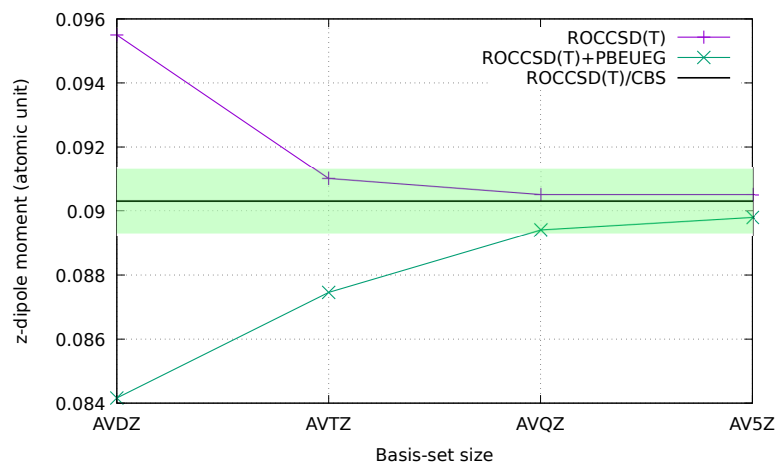

FIG. 2. BeH

TABLE IV. BF

| Basis/Method | HF      | CCSD(T) | CCSD(T)+PBEUEG |
|--------------|---------|---------|----------------|
| aug-cc-pVDZ  | 0.34436 | 0.34100 | 0.33287        |
| aug-cc-pVTZ  | 0.33390 | 0.32700 | 0.32351        |
| aug-cc-pVQZ  | 0.33314 | 0.32300 | 0.32082        |
| aug-cc-pV5Z  | 0.33328 | 0.32200 | 0.32068        |
| CBS          |         | 0.32081 |                |

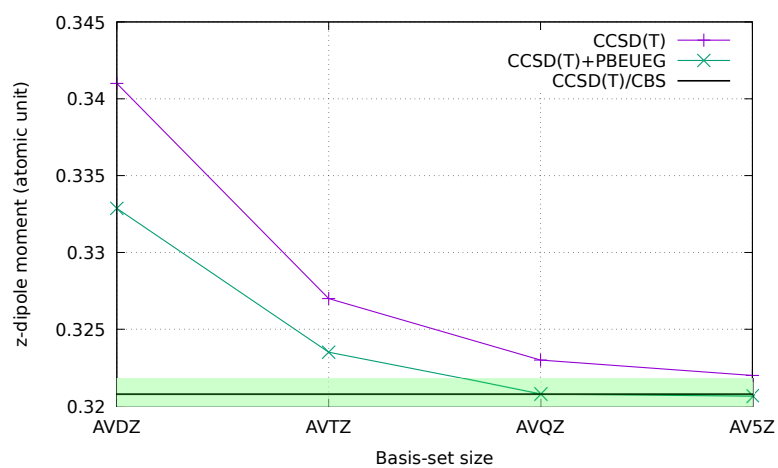

FIG. 3. BF

TABLE V. BH

| Basis/ Method | HF      | CCSD(T) | CCSD(T)+PBEUEG |
|---------------|---------|---------|----------------|
| aug-cc-pVDZ   | 0.68796 | 0.52950 | 0.54162        |
| aug-cc-pVTZ   | 0.68649 | 0.54500 | 0.55002        |
| aug-cc-pVQZ   | 0.68493 | 0.54750 | 0.54986        |
| aug-cc-pV5Z   | 0.68496 | 0.54850 | 0.54980        |
| CBS           |         | 0.54953 |                |

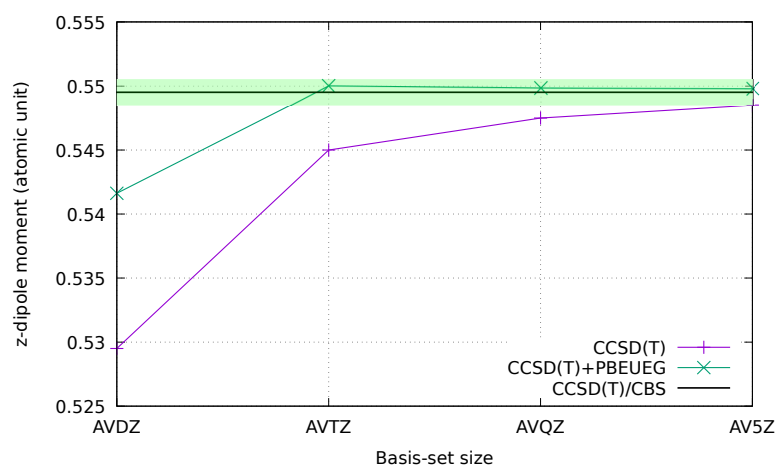

FIG. 4. BH

TABLE VI. CH

| Basis/Method | ROHF    | ROCCSD(T) | ROCCSD(T)+PBEUEG |
|--------------|---------|-----------|------------------|
| aug-cc-pVDZ  | 0.62348 | 0.54150   | 0.55427          |
| aug-cc-pVTZ  | 0.62000 | 0.54950   | 0.55481          |
| aug-cc-pVQZ  | 0.61871 | 0.55150   | 0.55405          |
| aug-cc-pV5Z  | 0.61858 | 0.55250   | 0.55396          |
| CBS          |         | 0.55368   |                  |

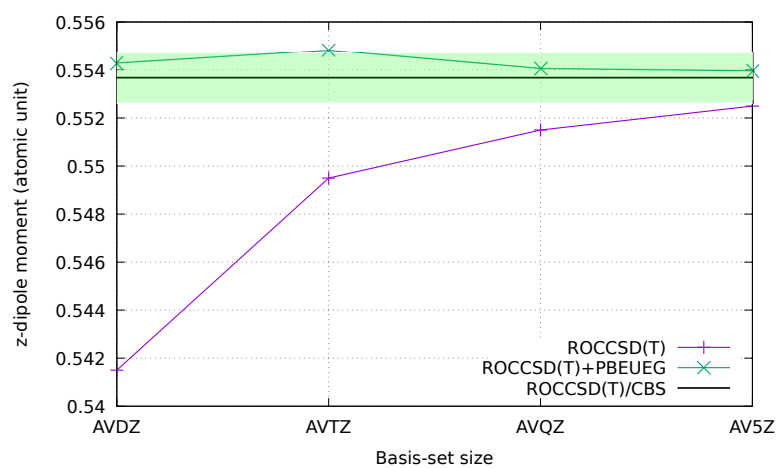

FIG. 5. CH

TABLE VII. NH

| Basis/Method | HF      | CCSD(T) | CCSD(T)+PBEUEG |
|--------------|---------|---------|----------------|
| aug-cc-pVDZ  | 0.63850 | 0.59350 | 0.60792        |
| aug-cc-pVTZ  | 0.63505 | 0.59950 | 0.60519        |
| aug-cc-pVQZ  | 0.63381 | 0.60200 | 0.60464        |
| aug-cc-pV5Z  | 0.63384 | 0.60350 | 0.60506        |
| CBS          |         | 0.60504 |                |

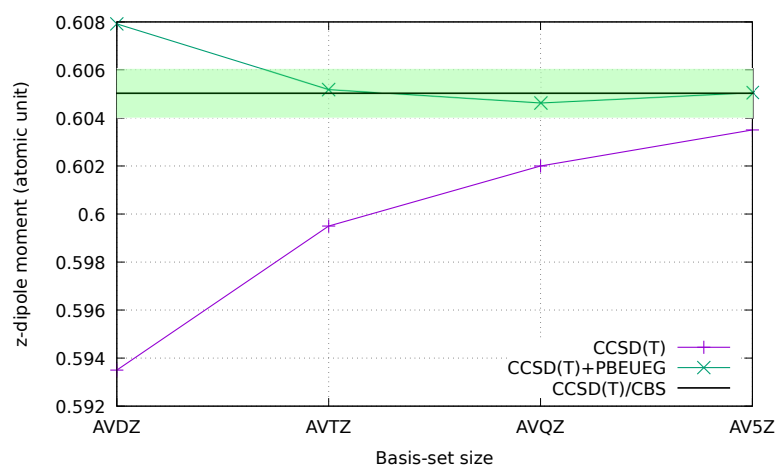

FIG. 6. NH

TABLE VIII. CH<sub>2</sub>

| Basis/Method | HF      | CCSD(T) | CCSD(T)+PBEUEG |
|--------------|---------|---------|----------------|
| aug-cc-pVDZ  | 0.74877 | 0.65600 | 0.66666        |
| aug-cc-pVTZ  | 0.74477 | 0.66000 | 0.66455        |
| aug-cc-pVQZ  | 0.74355 | 0.66200 | 0.66420        |
| aug-cc-pV5Z  | 0.74353 | 0.66350 | 0.66478        |
| CBS          |         | 0.66510 |                |

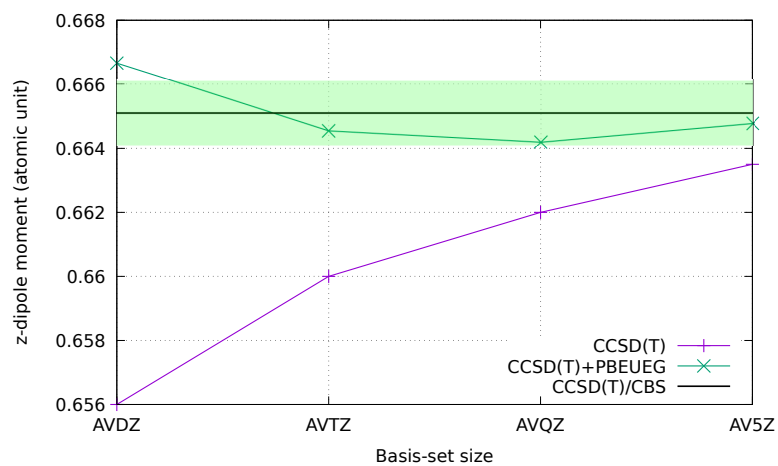FIG. 7. CH<sub>2</sub>

TABLE IX. FH

| Basis/Method | HF      | CCSD(T) | CCSD(T)+PBEUEG |
|--------------|---------|---------|----------------|
| aug-cc-pVDZ  | 0.75976 | 0.70350 | 0.71371        |
| aug-cc-pVTZ  | 0.75751 | 0.70450 | 0.70903        |
| aug-cc-pVQZ  | 0.75634 | 0.70700 | 0.70946        |
| aug-cc-pV5Z  | 0.75617 | 0.70750 | 0.70900        |
| CBS          |         | 0.70820 |                |

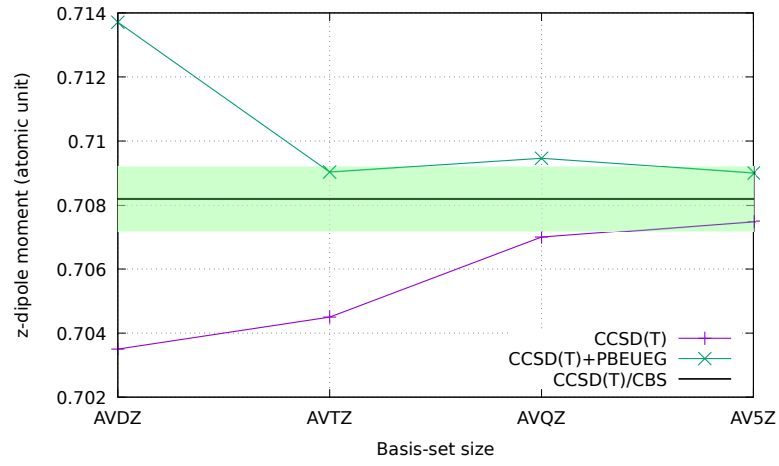

FIG. 8. FH

TABLE X. H<sub>2</sub>O

| Basis/Method | HF      | CCSD(T) | CCSD(T)+PBEUEG |
|--------------|---------|---------|----------------|
| aug-cc-pVDZ  | 0.78671 | 0.72700 | 0.73891        |
| aug-cc-pVTZ  | 0.78039 | 0.72400 | 0.72930        |
| aug-cc-pVQZ  | 0.77956 | 0.72650 | 0.72912        |
| aug-cc-pV5Z  | 0.77956 | 0.72800 | 0.72920        |
| CBS          |         | 0.72957 |                |

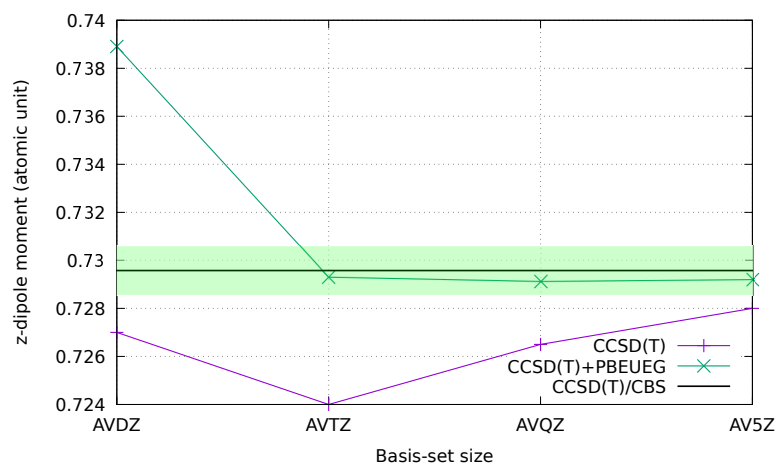FIG. 9. H<sub>2</sub>O

TABLE XI. BN

| Basis/Method | ROHF    | ROCCSD(T) | ROCCSD(T)+PBEUEG |
|--------------|---------|-----------|------------------|
| aug-cc-pVDZ  | 1.13451 | 0.76250   | 0.77517          |
| aug-cc-pVTZ  | 1.13862 | 0.77550   | 0.78145          |
| aug-cc-pVQZ  | 1.13831 | 0.78400   | 0.78756          |
| aug-cc-pV5Z  | 1.13840 | 0.78650   | 0.78846          |
| CBS          |         | 0.78902   |                  |

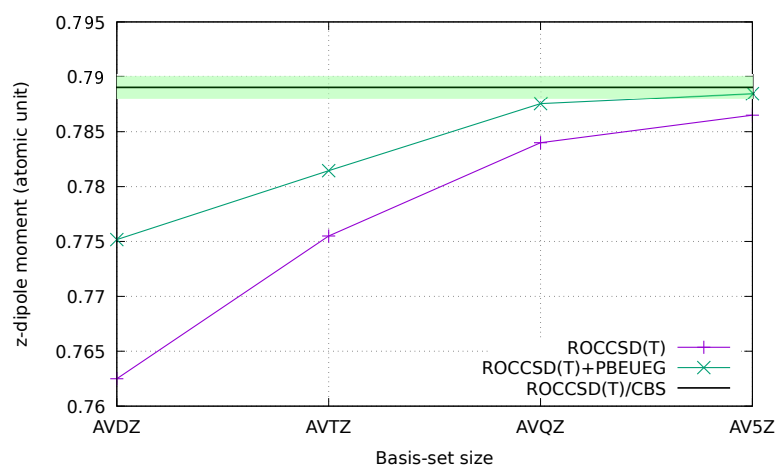

FIG. 10. BN

TABLE XII. BO

| Basis/Method | ROHF    | ROCCSD(T) | ROCCSD(T)+PBEUEG |
|--------------|---------|-----------|------------------|
| aug-cc-pVDZ  | 1.17803 | 0.88300   | 0.89417          |
| aug-cc-pVTZ  | 1.18533 | 0.89550   | 0.90153          |
| aug-cc-pVQZ  | 1.18527 | 0.90250   | 0.90622          |
| aug-cc-pV5Z  | 1.18539 | 0.90450   | 0.90698          |
| CBS          |         | 0.90647   |                  |

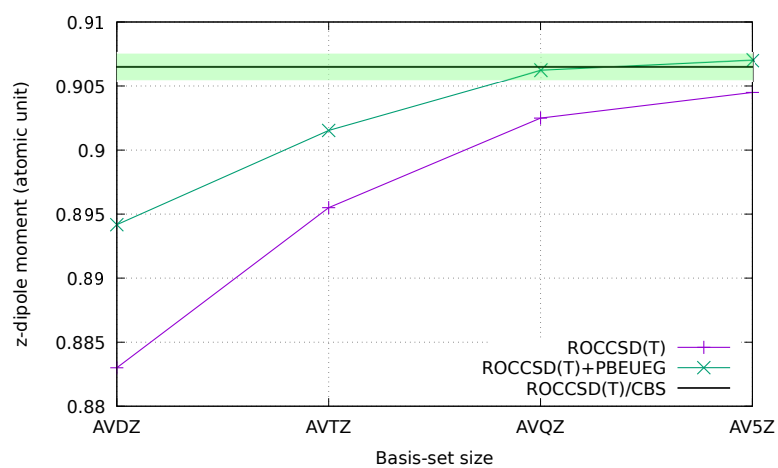

FIG. 11. BO

TABLE XIII. LiH

| Basis/Method | HF      | CCSD(T) | CCSD(T)+PBEUEG |
|--------------|---------|---------|----------------|
| aug-cc-pVDZ  | 2.37055 | 2.32500 | 2.32501        |
| aug-cc-pVTZ  | 2.36235 | 2.31000 | 2.30965        |
| aug-cc-pVQZ  | 2.36153 | 2.30800 | 2.30795        |
| aug-cc-pV5Z  | 2.36129 | 2.30800 | 2.30802        |
| CBS          |         | 2.30825 |                |

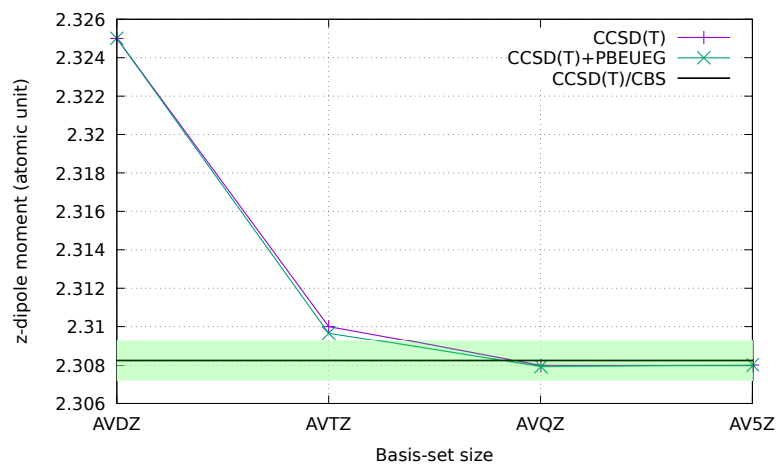

FIG. 12. LiH

TABLE XIV. LiF

| Basis/Method | HF      | CCSD(T) | CCSD(T)+PBEUEG |
|--------------|---------|---------|----------------|
| aug-cc-pVDZ  | 2.56111 | 2.50400 | 2.50942        |
| aug-cc-pVTZ  | 2.54103 | 2.48300 | 2.48542        |
| aug-cc-pVQZ  | 2.53949 | 2.48250 | 2.48367        |
| aug-cc-pV5Z  | 2.53905 | 2.48250 | 2.48321        |
| CBS          |         | 2.48297 |                |

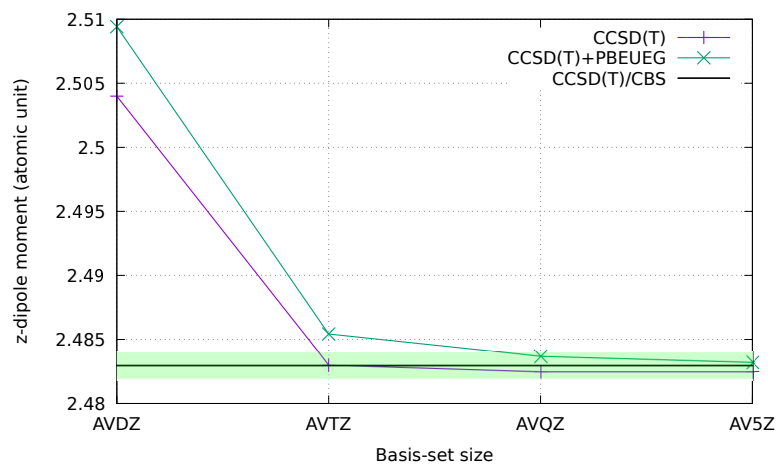

FIG. 13. LiF

TABLE XV. LiN

| Basis/Method | ROHF    | ROCCSD(T) | ROCCSD(T)+PBEUEG |
|--------------|---------|-----------|------------------|
| aug-cc-pVDZ  | 2.90309 | 2.74200   | 2.75215          |
| aug-cc-pVTZ  | 2.90379 | 2.77300   | 2.77714          |
| aug-cc-pVQZ  | 2.90372 | 2.78250   | 2.78464          |
| aug-cc-pV5Z  | 2.90317 | 2.78450   | 2.78583          |
| CBS          |         | 2.78718   |                  |

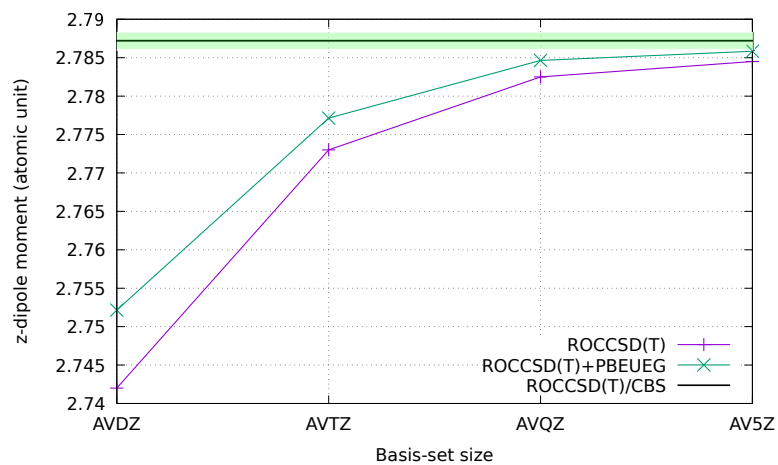

FIG. 14. LiN

### III. TABLE OF ERRORS

TABLE XVI. Errors in dipole moments (in atomic units) with respect to CCSD(T)/CBS for frozen-core calculations for the entire set of molecules. For each Dunning basis set (AVXZ=aug-cc-pVXZ,  $X \in \{D, T, Q, 5\}$ ), the first column contains the errors of the CCSD(T) dipole moments and the second column contains the errors after adding the PBEUEG basis-set correction.

|                           | AVDZ     |          | AVTZ     |          | AVQZ     |          | AV5Z     |          |
|---------------------------|----------|----------|----------|----------|----------|----------|----------|----------|
|                           | CCSD(T)  | +PBEUEG  | CCSD(T)  | +PBEUEG  | CCSD(T)  | +PBEUEG  | CCSD(T)  | +PBEUEG  |
| CO                        | 0.01065  | -0.00087 | 0.00515  | -0.00071 | 0.00115  | -0.00212 | 0.00065  | -0.00125 |
| BeH                       | 0.00520  | -0.00614 | 0.00070  | -0.00284 | 0.00020  | -0.00089 | 0.00020  | -0.00050 |
| BF                        | 0.02019  | 0.01207  | 0.00619  | 0.00270  | 0.00219  | 0.00001  | 0.00119  | -0.00013 |
| BH                        | 0.02003  | 0.00791  | 0.00453  | -0.00049 | 0.00203  | -0.00033 | 0.00103  | -0.00027 |
| CH                        | 0.01218  | -0.00059 | 0.00418  | -0.00112 | 0.00218  | -0.00036 | 0.00118  | -0.00027 |
| NH                        | 0.01154  | -0.00288 | 0.00554  | -0.00015 | 0.00304  | 0.00041  | 0.00154  | -0.00002 |
| CH <sub>2</sub> (singlet) | 0.00910  | -0.00156 | 0.00510  | 0.00055  | 0.00310  | 0.00090  | 0.00160  | 0.00032  |
| FH                        | 0.00470  | -0.00551 | 0.00370  | -0.00083 | 0.00120  | -0.00126 | 0.00070  | -0.00080 |
| H <sub>2</sub> O          | 0.00257  | -0.00934 | 0.00557  | 0.00027  | 0.00307  | 0.00045  | 0.00157  | 0.00037  |
| BN                        | 0.02652  | 0.013855 | 0.01352  | 0.00757  | 0.00502  | 0.00146  | 0.00252  | 0.00056  |
| BO                        | 0.02347  | 0.01230  | 0.01097  | 0.00494  | 0.00397  | 0.00025  | 0.00197  | -0.00051 |
| LiH                       | 0.01675  | 0.01676  | 0.00175  | 0.00140  | -0.00025 | -0.00030 | -0.00025 | -0.00023 |
| LiF                       | -0.02103 | -0.02645 | -0.00003 | -0.00246 | 0.00047  | -0.00070 | 0.00047  | -0.00024 |
| LiN                       | 0.04518  | 0.03504  | 0.01418  | 0.01004  | 0.00468  | 0.00254  | 0.00268  | 0.00136  |

TABLE XVII. Relative errors (%) in dipole moments with respect to CCSD(T)/CBS for frozen-core calculations for the entire set of molecules. For each Dunning basis set (AVXZ=aug-cc-pVXZ,  $X \in \{D, T, Q, 5\}$ ), the first column contains the errors of the CCSD(T) dipole moments and the second column contains the errors after adding the PBEUEG basis-set correction.

|                           | AVDZ    |         | AVTZ    |         | AVQZ    |         | AV5Z    |         |
|---------------------------|---------|---------|---------|---------|---------|---------|---------|---------|
|                           | CCSD(T) | +PBEUEG | CCSD(T) | +PBEUEG | CCSD(T) | +PBEUEG | CCSD(T) | +PBEUEG |
| CO                        | 23.75   | -1.95   | 11.48   | -1.59   | 2.57    | -4.74   | 1.45    | -2.80   |
| BeH                       | 5.76    | -6.79   | 0.78    | -3.14   | 0.22    | -0.99   | 0.22    | -0.56   |
| BF                        | 6.29    | 3.76    | 1.93    | 0.84    | 0.68    | 0.00    | 0.37    | -0.04   |
| BH                        | -3.64   | -1.44   | -0.82   | 0.09    | -0.37   | 0.06    | -0.19   | 0.05    |
| CH                        | -2.20   | 0.11    | -0.76   | 0.20    | -0.39   | 0.07    | -0.21   | 0.05    |
| NH                        | -1.91   | 0.48    | -0.92   | 0.02    | -0.50   | -0.07   | -0.25   | 0.00    |
| CH <sub>2</sub> (singlet) | -1.37   | 0.23    | -0.77   | -0.08   | -0.47   | -0.14   | -0.24   | -0.05   |
| FH                        | -0.66   | 0.78    | -0.52   | 0.12    | -0.17   | 0.18    | -0.10   | 0.11    |
| H <sub>2</sub> O          | -0.35   | 1.28    | -0.76   | -0.04   | -0.42   | -0.06   | -0.22   | -0.05   |
| BN                        | -3.36   | -1.76   | -1.71   | -0.96   | -0.64   | -0.19   | -0.32   | -0.07   |
| BO                        | -2.59   | -1.36   | -1.21   | -0.55   | -0.44   | -0.03   | -0.22   | 0.06    |
| LiH                       | 0.73    | 0.73    | 0.08    | 0.06    | -0.01   | -0.01   | -0.01   | -0.01   |
| LiF                       | 0.85    | 1.07    | 0.00    | 0.10    | -0.02   | 0.03    | -0.02   | 0.01    |
| LiN                       | -1.62   | -1.26   | -0.51   | -0.36   | -0.17   | -0.09   | -0.10   | -0.05   |

- [1] D. Hait and M. Head-Gordon, *Journal of Chemical Theory and Computation* **14**, 1969 (2018).  
 [2] A. Halkier, W. Klopper, T. Helgaker and P. Jorgensen, *J. Chem. Phys.* **111**, 4424 (1999).
